# Supplementary material for: Closed-form survival probabilities for biased random walks at arbitrary step number
Source: arXiv:2505.24814 ancillary file (2025-05-30)
Supplement: Supplementary file 1 [file SupplMat.pdf]

# Supplemental Material –
# Closed-form survival probabilities for biased random walks at arbitrary step number

Debendro Mookerjee and Sarah Kostinski†

## Derivation of the Survival Probability $R(N)$

The survival probability $R(N)$ is defined as the probability to remain to the right of the target $x_b = -m$. In Eq. 2 of the main text, we showed that it is given by

$$R(N) = \sum_{\{n,k\}} p^n q^k C_m(n,k) = \sum_k p^{N-k} q^k C_m(N-k,k)$$
$$= \sum_{k=0}^{N} p^{N-k} q^k C_m(N-k,k) \tag{S1}$$

where $n$ denotes the number of steps to the right, and $k = N - n$ denotes the number of steps to the left. To evaluate the sum, we must consider three possible scenarios: $m > N$, $N = m$, and $m < N$. The first two are explained in the main text and thus we confine our attention here to the third scenario ($m < N$). The Catalan trapezoids are defined as[1]

$$C_m(n,k) = \begin{cases} \binom{n+k}{k} & 0 \le k < m \\ \binom{n+k}{k} - \binom{n+k}{k-m} & m \le k \le n+m-1 \\ 0 & k > n+m-1\,. \end{cases} \tag{S2}$$

Accounting for both the $0 \le k < m$ and $m \le k \le n+m-1$ cases of the Catalan trapezoids yields

$$R(N) = \sum_{k=0}^{m-1} p^{N-k} q^k \binom{N}{k} + \sum_{k=m}^{n+m-1} p^{N-k} q^k \left[\binom{N}{k} - \binom{N}{k-m}\right] = \sum_{k=0}^{n+m-1} p^{N-k} q^k \binom{N}{k} - \sum_{k=m}^{n+m-1} p^{N-k} q^k \binom{N}{k-m} \tag{S3}$$

For both summations, $k \le n + m - 1$. Furthermore, because $N = n + k$, we can rewrite the inequality as

$$k \le N - k + m - 1 \qquad \longrightarrow \qquad k \le \frac{N+m-1}{2}\,. \tag{S4}$$

Since $k$ must be an integer, the inequality becomes:

$$k \le \left\lfloor \frac{N+m-1}{2} \right\rfloor. \tag{S5}$$

Eq. S3 thus simplifies to:

$$R(N) = \sum_{k=0}^{\lfloor \frac{N+m-1}{2} \rfloor} p^{N-k} q^k \binom{N}{k} - \sum_{k=m}^{\lfloor \frac{N+m-1}{2} \rfloor} p^{N-k} q^k \binom{N}{k-m}. \tag{S6}$$

We now prove two important identities that will be used to produce an analytic expression for $R(N)$ in terms of hypergeometric functions. The first identity is:

$$\sum_{\ell=0}^{k} x^\ell \binom{2k+m}{\ell} = (1+x)^{2k+m} - x^{k+1} \binom{2k+m}{k+1} {}_2F_1\big(1; 1-k-m; k+2; -x\big). \tag{S7}$$

†Department of Physics, New York University, New York, USA

**Proof:**
Beginning from the binomial theorem,

$$\begin{aligned}
\sum_{\ell=0}^{k} x^{\ell}\binom{2k+m}{\ell} &= (1+x)^{2k+m} - \sum_{\ell=k+1}^{2k+m} x^{\ell}\binom{2k+m}{\ell} = (1+x)^{2k+m} - x^{k+1}\sum_{\ell=k+1}^{2k+m} x^{\ell-k-1}\binom{2k+m}{\ell} \\
&= (1+x)^{2k+m} - x^{k+1}\sum_{n=0}^{k+m-1} x^{n}\binom{2k+m}{n+k+1} = (1+x)^{2k+m} - x^{k+1}\sum_{n=0}^{k+m-1} x^{n}\frac{(2k+m)!}{(n+k+1)!(k+m-n-1)!} \\
&= (1+x)^{2k+m} - x^{k+1}\sum_{n=0}^{k+m-1} x^{n}\frac{(2k+m)!}{(n+k+1)!(k+m-n-1)!}\binom{2k+m}{k+1}\frac{(k+1)!(k+m-1)!}{(2k+m)!} \\
&= (1+x)^{2k+m} - x^{k+1}\binom{2k+m}{k+1}\sum_{n=0}^{k+m-1} x^{n}\frac{(k+1)!(k+m-1)!}{(n+k+1)!(k+m-n-1)!} \\
&= (1+x)^{2k+m} - x^{k+1}\binom{2k+m}{k+1}\sum_{n=0}^{k+m-1} \frac{(-x)^{n}(-1)^{n}}{n!}n!\frac{(k+m-1)(k+m-2)...(k+m-n)}{(n+k+1)(n+k)...(k+2)} \\
&= (1+x)^{2k+m} - x^{k+1}\binom{2k+m}{k+1}\sum_{n=0}^{k+m-1} \frac{(-x)^{n}}{n!}n!\frac{(1-k-m)(2-k-m)...(n-m-k)}{(n+k+1)(n+k)...(k+2)} \\
&= (1+x)^{2k+m} - x^{k+1}\binom{2k+m}{k+1}\sum_{n=0}^{k+m-1} \frac{(1)_n(1-k-m)_n}{(k+2)_n}\frac{(-x)^{n}}{n!} \\
&= (1+x)^{2k+m} - x^{k+1}\binom{2k+m}{k+1}{}_2F_1\big(1;1-k-m;k+2;-x\big) \qquad \spadesuit
\end{aligned}$$

The second identity is:

$$\sum_{\ell=0}^{k-1} x^{\ell}\binom{2k-m}{\ell} = (1+x)^{2k-m} - x^{k}\binom{2k-m}{k}{}_2F_1\big(1;m-k;k+1;-x\big). \tag{S8}$$

**Proof:**

$$\begin{aligned}
\sum_{\ell=0}^{k-1} x^{\ell}\binom{2k-m}{\ell} &= (1+x)^{2k-m} - \sum_{\ell=k}^{2k-m} x^{\ell}\binom{2k-m}{\ell} = (1+x)^{2k-m} - x^{k}\sum_{\ell=k}^{2k-m} x^{\ell-k}\binom{2k-m}{\ell} \\
&= (1+x)^{2k-m} - x^{k}\sum_{n=0}^{k-m} x^{n}\binom{2k-m}{n+k} = (1+x)^{2k-m} - x^{k}\sum_{n=0}^{k-m} x^{n}\frac{(2k-m)!}{(n+k)!(k-m-n)!} \\
&= (1+x)^{2k-m} - x^{k}\sum_{n=0}^{k-m} x^{n}\frac{(2k-m)!}{(n+k)!(k-m-n)!}\binom{2k-m}{k}\frac{k!(k-m)!}{(2k-m)!} \\
&= (1+x)^{2k-m} - x^{k}\binom{2k-m}{k}\sum_{n=0}^{k-m} x^{n}\frac{k!(k-m)!}{(n+k)!(k-m-n)!} \\
&= (1+x)^{2k-m} - x^{k}\binom{2k-m}{k}\sum_{n=0}^{k-m} \frac{(-x)^{n}(-1)^{n}}{n!}n!\frac{(k-m)(k-m-1)...(k-m-n+1)}{(n+k)(n+k-1)...(k+1)} \\
&= (1+x)^{2k-m} - x^{k}\binom{2k-m}{k}\sum_{n=0}^{k-m} \frac{(-x)^{n}}{n!}n!\frac{(m-k)(1+m-k)...(m+n-k-1)}{(n+k)(n+k-1)...(k+1)} \\
&= (1+x)^{2k-m} - x^{k}\binom{2k-m}{k}\sum_{n=0}^{k-m} \frac{(1)_n(m-k)_n}{(k+1)_n}\frac{(-x)^{n}}{n!} \\
&= (1+x)^{2k-m} - x^{k}\binom{2k-m}{k}{}_2F_1\big(1;m-k;k+1;-x\big) \qquad \spadesuit
\end{aligned}$$

In order to use these two derived hypergeometric identities, we rewrite the survival probability $R(N)$ as follows:

$$\begin{aligned} R(N) &= \sum_{k=0}^{\lfloor\frac{N+m-1}{2}\rfloor} p^{N-k}q^k\binom{N}{k} - \sum_{k=m}^{\lfloor\frac{N+m-1}{2}\rfloor} p^{N-k}q^k\binom{N}{k-m} \\ &= p^N \sum_{k=0}^{\lfloor\frac{N+m-1}{2}\rfloor}\left(\frac{q}{p}\right)^k\binom{N}{k} - p^N \sum_{\ell=0}^{\lfloor\frac{N+m-1}{2}\rfloor-m}\left(\frac{q}{p}\right)^{\ell+m}\binom{N}{\ell} \\ &\equiv p^N \sum_{\ell=0}^{\lfloor\frac{N+m-1}{2}\rfloor}\gamma^\ell\binom{N}{\ell} - p^{N-m}q^m \sum_{\ell=0}^{\lfloor\frac{N+m-1}{2}\rfloor-m}\gamma^\ell\binom{N}{\ell} \end{aligned} \tag{S9}$$

where $\gamma \equiv q/p$. Examining the first sum of the expression, we consider two cases: $N+m = 2k$ and $N+m = 2k+1$. These cases correspond to even and odd $N+m$, respectively. In the case $N+m=2k$, we obtain

$$\sum_{\ell=0}^{\lfloor\frac{N+m-1}{2}\rfloor}\gamma^\ell\binom{N}{\ell} = \sum_{\ell=0}^{k-1}\gamma^\ell\binom{2k-m}{\ell} = (1+\gamma)^{2k-m} - \gamma^k\binom{2k-m}{k}{}_2F_1\big(1;m-k;k+1;-\gamma\big), \tag{S10}$$

while for the latter case $N+m = 2k+1$, we have

$$\begin{aligned} \sum_{\ell=0}^{\lfloor\frac{N+m-1}{2}\rfloor}\gamma^\ell\binom{N}{\ell} &= \sum_{\ell=0}^{k}\gamma^\ell\binom{2k-m+1}{\ell} = \sum_{\ell=0}^{k-1}\gamma^\ell\binom{2k-(m-1)}{\ell} + \gamma^k\binom{2k-m+1}{k} \\ &= (1+\gamma)^{2k-m+1} - \gamma^k\binom{2k-m+1}{k}{}_2F_1\big(1;m-1-k;k+1;-\gamma\big) + \gamma^k\binom{2k-m+1}{k}, \end{aligned} \tag{S11}$$

where in both cases we used the second identity (Eq. S8). Thus, the first sum of Eq. S9 becomes

$$\sum_{\ell=0}^{\lfloor\frac{N+m-1}{2}\rfloor}\gamma^\ell\binom{N}{\ell} = \begin{cases} (1+\gamma)^{2k-m} - \gamma^k\binom{2k-m}{k}{}_2F_1\big(1;m-k;k+1;-\gamma\big) & N+m=2k \\ (1+\gamma)^{2k-m+1} - \gamma^k\binom{2k-m+1}{k}{}_2F_1\big(1;m-1-k;k+1;-\gamma\big) + \gamma^k\binom{2k-m+1}{k} & N+m=2k+1 \end{cases} \tag{S12}$$

For the final sum of Eq. S9, we will again consider the two cases $N+m=2k$ and $N+m=2k+1$. In the former case, we obtain

$$\begin{aligned} \sum_{\ell=0}^{\lfloor\frac{N+m-1}{2}\rfloor-m}\gamma^\ell\binom{N}{\ell} &= \sum_{\ell=0}^{(k-m)-1}\gamma^\ell\binom{2k-m}{\ell} = \sum_{\ell=0}^{(k-m)-1}\gamma^\ell\binom{2(k-m)+m}{\ell} \\ &= \sum_{\ell=0}^{k-m}\gamma^\ell\binom{2(k-m)+m}{\ell} - \gamma^{k-m}\binom{2k-m}{k-m} \\ &= (1+\gamma)^{2k-m} - \gamma^{k-m+1}\binom{2k-m}{k-m+1}{}_2F_1\big(1;1-k;k-m+2;-\gamma\big) - \gamma^{k-m}\binom{2k-m}{k-m} \end{aligned} \tag{S13}$$

where we used the first identity (Eq. S7). In the latter case ($N+m=2k+1$), we obtain

$$\begin{aligned} \sum_{\ell=0}^{\lfloor\frac{N+m-1}{2}\rfloor-m}\gamma^\ell\binom{N}{\ell} &= \sum_{\ell=0}^{k-m}\gamma^\ell\binom{2k-m+1}{\ell} = \sum_{\ell=0}^{k-m}\gamma^\ell\binom{2(k-m)+(m+1)}{\ell} \\ &= (1+\gamma)^{2k-m+1} - \gamma^{k-m+1}\binom{2k-m+1}{k-m+1}{}_2F_1\big(1;-k;k-m+2;-\gamma\big). \end{aligned} \tag{S14}$$

Thus the final sum of Eq. S9 becomes:

$$\sum_{\ell=0}^{\lfloor\frac{N+m-1}{2}\rfloor-m}\gamma^\ell\binom{N}{\ell} = \begin{cases} (1+\gamma)^{2k-m} - \gamma^{k-m+1}\binom{2k-m}{k-m+1}{}_2F_1\big(1;1-k;k-m+2;-\gamma\big) - \gamma^{k-m}\binom{2k-m}{k-m} & N+m=2k \\ (1+\gamma)^{2k-m+1} - \gamma^{k-m+1}\binom{2k-m+1}{k-m+1}{}_2F_1\big(1;-k;k-m+2;-\gamma\big) & N+m=2k+1 \end{cases} \tag{S15}$$

Eq. S9 can then be written in closed form as:

$$R(N) = p^N \sum_{\ell=0}^{\lfloor \frac{N+m-1}{2} \rfloor} \gamma^\ell \binom{N}{\ell} - p^{N-m} q^m \sum_{\ell=0}^{\lfloor \frac{N+m-1}{2} \rfloor - m} \gamma^\ell \binom{N}{\ell} \tag{S16}$$

$$= p^N \begin{cases} (1+\gamma)^{2k-m} - \gamma^k \binom{2k-m}{k} {}_2F_1\big(1; m-k; k+1; -\gamma\big) & N+m=2k \\ (1+\gamma)^{2k-m+1} - \gamma^k \binom{2k-m+1}{k} {}_2F_1\big(1; m-1-k; k+1; -\gamma\big) + \gamma^k \binom{2k-m+1}{k} & N+m=2k+1 \end{cases}$$

$$- p^{N-m} q^m \begin{cases} (1+\gamma)^{2k-m} - \gamma^{k-m+1} \binom{2k-m}{k-m+1} {}_2F_1\big(1; 1-k; k-m+2; -\gamma\big) - \gamma^{k-m} \binom{2k-m}{k-m} & N+m=2k \\ (1+\gamma)^{2k-m+1} - \gamma^{k-m+1} \binom{2k-m+1}{k-m+1} {}_2F_1\big(1; -k; k-m+2; -\gamma\big) & N+m=2k+1 \end{cases} \tag{S17}$$

To simplify this formula, let us first consider the case $N+m=2k$. The corresponding survival probability $R(N)$ is

$$R(N) = p^N \Big[(1+\gamma)^N - \gamma^{\frac{N+m}{2}} \binom{N}{\frac{N+m}{2}} {}_2F_1\Big(1; \frac{m-N}{2}; \frac{N+m+2}{2}; -\gamma\Big)\Big] - p^{N-m} q^m \Big[(1+\gamma)^N - \gamma^{\frac{N-m}{2}} \binom{N}{\frac{N-m}{2}}$$
$$- \gamma^{\frac{N-m+2}{2}} \binom{N}{\frac{N-m+2}{2}} {}_2F_1\Big(1; \frac{2-N-m}{2}; \frac{N-m+4}{2}; -\gamma\Big)\Big]. \tag{S18}$$

The terms involving $(1+\gamma)^N$ can be grouped and further simplified as

$$(1+\gamma)^N (p^N - p^{N-m} q^m) = p^N (1+\gamma)^N (1-\gamma^m) = (p+q)^N (1-\gamma^m) = 1-\gamma^m\,. \tag{S19}$$

The survival probability thus becomes

$$R(N) = 1 - \gamma^m + \gamma^{\frac{N+m}{2}} p^N \binom{N}{\frac{N-m}{2}}$$
$$- p^N \gamma^{\frac{N+m}{2}} \binom{N}{\frac{N+m}{2}} {}_2F_1\Big(1; \frac{m-N}{2}; \frac{N+m+2}{2}; -\gamma\Big) + p^N \gamma^{\frac{N+m}{2}} \gamma \binom{N}{\frac{N-m+2}{2}} {}_2F_1\Big(1; \frac{2-N-m}{2}; \frac{N-m+4}{2}; -\gamma\Big). \tag{S20}$$

Noting that $\binom{N}{\frac{N-m}{2}} = \binom{N}{\frac{N+m}{2}}$ leads to the following expression for the survival probability when $N+m$ is even:

$$R_e(N) = 1 - \gamma^m + \gamma^{\frac{N+m}{2}} p^N \binom{N}{\frac{N-m}{2}} \Big[1 - {}_2F_1\Big(1; \frac{m-N}{2}; \frac{N+m+2}{2}; -\gamma\Big)\Big] + p^N \gamma^{\frac{N+m}{2}} \gamma \binom{N}{\frac{N-m+2}{2}} {}_2F_1\Big(1; \frac{2-N-m}{2}; \frac{N-m+4}{2}; -\gamma\Big) \tag{S21}$$

where the subscript $e$ of $R_e(N)$ serves as a reminder that $N+m$ is even. A similar procedure simplifies the survival probability expression when $N+m$ is odd, leading to the following:

$$R_o(N) = 1 - \gamma^m + \gamma^{\frac{N+m-1}{2}} p^N \binom{N}{\frac{N+m-1}{2}} \Big[1 - {}_2F_1\Big(1; \frac{m-N-1}{2}; \frac{N+m+1}{2}; -\gamma\Big)\Big]$$
$$+ p^N \gamma^{\frac{N+m+1}{2}} \binom{N}{\frac{N-m+1}{2}} {}_2F_1\Big(1; \frac{1-N-m}{2}; \frac{N-m+3}{2}; -\gamma\Big). \tag{S22}$$

## Behavior of $R(N)$ in the large $N$ limit when $\gamma \equiv q/p < 1$

Without loss of generality, let us consider the case when $N+m=2k$. The survival probability $R(N)$ in this case is given by Eq. S21. In the limit of large $N$ where $N \gg m$, the two binomial coefficients appearing in Eq. S21 can be approximated as

$$\binom{N}{\frac{N-m}{2}} \approx \binom{N}{\frac{N-m+2}{2}} \approx \binom{N}{\frac{N}{2}} = \frac{N!}{\left(\frac{N}{2}\right)! \left(\frac{N}{2}\right)!}\,. \tag{S23}$$

Furthermore, Stirling's approximation can be employed in the limit of large $N$:

$$\binom{N}{\frac{N-m}{2}} \approx \binom{N}{\frac{N-m+2}{2}} \approx \binom{N}{\frac{N}{2}} \approx 2^N \sqrt{\frac{2}{\pi N}}\,. \tag{S24}$$

Therefore, the survival probability takes on the approximate form

$$R(N) \approx 1 - \gamma^m + \gamma^{\frac{m}{2}} \left(2p\sqrt{\gamma}\right)^N \sqrt{\frac{2}{\pi N}} \left[1 - {}_2F_1\left(1; \frac{m-N}{2}; \frac{N+m+2}{2}; -\gamma\right)\right]$$
$$+ \gamma^{\frac{m}{2}} \gamma \left(2p\sqrt{\gamma}\right)^N \sqrt{\frac{2}{\pi N}} {}_2F_1\left(1; \frac{2-N-m}{2}; \frac{N-m+4}{2}; -\gamma\right). \tag{S25}$$

Since $p + q = 1$ and $q = \gamma p$, we find that

$$\left(2p\sqrt{\gamma}\right)^N = \left(\frac{2\sqrt{\gamma}}{\gamma+1}\right)^N . \tag{S26}$$

We see that the quantity inside the brackets is less than 1 except for the case $\gamma = 1$ (i.e. a symmetric walk where $p = q$). Thus, in the limit of large $N$, the quantity $\left(2p\sqrt{\gamma}\right)^N$ approaches zero for a biased walk ($p \neq q$ or when $\gamma < 1$). Let us now focus on the hypergeometric functions in the limit of large $N$. We note that the first hypergeometric function in Eq. S25 is the following:

$${}_2F_1\left(1; \frac{m-N}{2}; \frac{N+m+2}{2}; -\gamma\right) = \sum_{n=0}^{\infty} \frac{\left(\frac{m-N}{2}\right)_n}{\left(\frac{N+m+2}{2}\right)_n} (-\gamma)^n . \tag{S27}$$

For any positive integer $n$, $\left|(-\gamma)^n\right| < 1$ when $\gamma < 1$. We now examine the ratio of Pochhammer symbols, noting that the Pochhammer symbol $(x)_n$ is defined as $(x)(x+1)\cdots(x+n-1)$. Since $\left|\frac{m-N}{2}\right| < \left|\frac{N+m+2}{2}\right|$,

$$\left|\frac{\left(\frac{m-N}{2}\right)_n}{\left(\frac{N+m+2}{2}\right)_n}\right| = \left|\frac{\left(\frac{m-N}{2}\right)\left(\frac{m-N}{2}+1\right)\cdots\left(\frac{m-N}{2}+n-1\right)}{\left(\frac{N+m+2}{2}\right)\left(\frac{N+m+2}{2}+1\right)\cdots\left(\frac{N+m+2}{2}+n-1\right)}\right| < 1 \tag{S28}$$

Thus, the magnitude of the summands in Eq. S27 are all less than 1 (with the exception of the $n = 0$ term, which yields 1). Therefore,

$$\lim_{N\to\infty} \gamma^{\frac{m}{2}} \left(2p\sqrt{\gamma}\right)^N \sqrt{\frac{2}{\pi N}} \left[1 - {}_2F_1\left(1; \frac{m-N}{2}; \frac{N+m+2}{2}; -\gamma\right)\right] = 0 . \tag{S29}$$

Finally, we consider the term containing the remaining hypergeometric function in Eq. S25. This term is

$$\gamma^{\frac{m}{2}} \gamma \left(2p\sqrt{\gamma}\right)^N \sqrt{\frac{2}{\pi N}} {}_2F_1\left(1; \frac{2-N-m}{2}; \frac{N-m+4}{2}; -\gamma\right) = \gamma^{\frac{m}{2}+1} \sqrt{\frac{2}{\pi}} \sum_{n=0}^{\infty} \frac{\left(\frac{2-N-m}{2}\right)_n}{\left(\frac{N-m+4}{2}\right)_n} \frac{\left(\frac{2\sqrt{\gamma}}{\gamma+1}\right)^N}{\sqrt{N}} (-\gamma)^n \tag{S30}$$

When $\gamma$ is less than unity, we see that the quantity $\frac{1}{\sqrt{N}}\left(\frac{2\sqrt{\gamma}}{1+\gamma}\right)^N (-\gamma)^n$ multiplying the ratio of Pochhammer symbols in the summand goes to zero in the limit of large $N$. We also see that the ratio of Pochhammer symbols $\frac{\left(\frac{2-N-m}{2}\right)_n}{\left(\frac{N-m+4}{2}\right)_n}$ can be interpreted as the ratio of two $n$th-degree polynomials in $N$. This ratio is of the form $\frac{\pm N^n + \ldots}{N^n + \ldots}$, whose magnitude approaches unity as $N$ goes to infinity. Hence, we see that

$$\lim_{N\to\infty} \gamma^{\frac{m}{2}} \gamma \left(2p\sqrt{\gamma}\right)^N \sqrt{\frac{2}{\pi N}} {}_2F_1\left(1; \frac{2-N-m}{2}; \frac{N-m+4}{2}; -\gamma\right) = 0 . \tag{S31}$$

These observations reveal that when $\gamma < 1$,

$$\lim_{N\to\infty} R(N) = 1 - \gamma^m . \tag{S32}$$

## Probability of last passage (PLP)

Let us define the probability of last passage (PLP) as the probability to visit $x_b = -m$ for the last time at step $n$, where $n > m$. For a total walk length of $N$ steps, this probability can be expressed as:

$$PLP = (\text{probability to be at } x_b = -m \text{ at step } n) \times (\text{probability of surviving } N-n \text{ steps thereafter})$$

To derive an expression for the PLP, let us first consider a path that takes the random walker from the origin to the target $x_b = -m$. Let the number of steps taken to the right and left be $n_R$ and $n_L$, respectively. Thus $n_L = n_R + m$. We then have the following two equations: $n_L - n_R = m$ and $n_L + n_R = n$, which can be simplified as

$$n_L = \frac{n+m}{2} \tag{S33}$$

$$n_R = \frac{n-m}{2}\,. \tag{S34}$$

Note that $n_L$ and $n_R$ must be integers, where last passage occurs only when $n+m$ and $n-m$ are even. The probability of such a path occurring is $p^{\frac{n-m}{2}} q^{\frac{n+m}{2}}$. Furthermore, the total number of such paths is $\binom{n}{n_R} = \binom{n}{\frac{n-m}{2}}$. Thus,

$$PLP = p^{\frac{n-m}{2}} q^{\frac{n+m}{2}} \binom{n}{\frac{n-m}{2}} \times S(N-n) \tag{S35}$$

where $S(N-n)$ is the survival probability. Here $S(N-n)$ is equivalent to the complement of the recurrence (return) probability, since $x_b$ serves as both the point of origin and the target of the remainder of the random walk after step $n$. We can thus use results for the survival probability in the recurrence problem[2]:

$$S_{\text{odd}}(N,B) = B + \frac{(1-B^2)^{\frac{N}{2}}}{2^{N-1}} \binom{N-1}{\frac{N-1}{2}} \sqrt{\frac{1-B}{1+B}} \left[1 - \frac{2B}{1+B}\,\frac{N-1}{N+1}\,{}_2F_1\!\left(1; -\frac{N}{2}+\frac{3}{2}; \frac{N}{2}+\frac{3}{2}; \frac{B-1}{B+1}\right)\right] \tag{S36}$$

$$S_{\text{even}}(N,B) = B + \frac{(1-B^2)^{\frac{N}{2}}}{2^{N}} \binom{N}{\frac{N}{2}} \left[\frac{1-B}{1+B} - 2B\,\frac{1-B}{(1+B)^2}\,\frac{N-2}{N+2}\,{}_2F_1\!\left(1; -\frac{N}{2}+2; \frac{N}{2}+2; \frac{B-1}{B+1}\right)\right] \tag{S37}$$

where $S_{\text{odd}}$ should be used if $N-n$ is odd, and $S_{\text{even}}$ should be used if $N-n$ is even. When combined with Eq. S35, this yields the full expression for the PLP.

## Critical bias for a monotonically decaying PLP tail

Here we derive the critical bias expressions given in the main text. Note that because last passage can only occur when $n+m$ is even, the probability of last passage alternates between zero and nonzero values for consecutive step numbers. Therefore, we concern ourselves here only with nonzero values of the PLP, i.e. for the case when $n+m$ is even-valued. Below we study two possible scenarios, i.e. when $N+m$ is even and when $N+m$ is odd.

### Case 1: $N+m$ is even

To determine the critical bias beyond which the nonzero PLP values decrease monotonically we require that

$$PLP(N-2) - PLP(N) > 0 \tag{S38}$$

where $PLP(N) = p^{\frac{N-m}{2}} q^{\frac{N+m}{2}} \binom{N}{\frac{N-m}{2}}$. Because $p = \frac{1+B}{2}$ and $q = \frac{1-B}{2}$, this expression becomes

$$PLP(N) = \frac{1}{2^N}(1-B^2)^{\frac{N}{2}} \left(\frac{1-B}{1+B}\right)^{\frac{m}{2}} \binom{N}{\frac{N-m}{2}}. \tag{S39}$$

Meanwhile, $PLP(N-2)$ is equal to

$$PLP(N-2) = p^{\frac{N-m-2}{2}} q^{\frac{N+m-2}{2}} \binom{N-2}{\frac{N-m-2}{2}} S(2) = \frac{1}{2^N}\,\frac{4}{1-B^2} \left(\frac{1-B}{1+B}\right)^{\frac{m}{2}} \binom{N-2}{\frac{N-m-2}{2}} (1-B^2)^{\frac{N}{2}}\, S(2)\,. \tag{S40}$$

Upon cancellation of common terms, the condition $PLP(N-2) - PLP(N) > 0$ becomes

$$\frac{4}{1-B^2}\binom{N-2}{\frac{N-m}{2}-1}S(2) - \binom{N}{\frac{N-m}{2}} > 0\,. \tag{S41}$$

We now rewrite the binomial coefficients as

$$\binom{N-2}{\frac{N-m}{2}-1} = \frac{(N-2)!}{\left(\frac{N+m-2}{2}\right)!\left(\frac{N-m-2}{2}\right)!} \tag{S42}$$

and

$$\binom{N}{\frac{N-m}{2}} = \frac{N!}{\left(\frac{N+m}{2}\right)!\left(\frac{N-m}{2}\right)!} = \frac{N(N-1)}{\left(\frac{N+m}{2}\right)\left(\frac{N-m}{2}\right)}\binom{N-2}{\frac{N-m}{2}-1}. \tag{S43}$$

Substituting these into Eq. S41 yields

$$\frac{S(2)}{1-B^2} - \frac{N(N-1)}{(N-m)(N+m)} > 0 \quad\longrightarrow\quad 1-B^2 < S(2)\left[\frac{N^2-m^2}{N(N-1)}\right]. \tag{S44}$$

Furthermore, one can show that $S(2) = p^2 + q^2 = \frac{1}{2}(1+B^2)$. Substituting into the above inequality gives

$$B^2 > \frac{N^2-2N+m^2}{3N^2-2N-m^2}\,, \tag{S45}$$

from which we obtain the condition given in the main text:

$$|B| > \sqrt{\frac{N^2-2N+m^2}{3N^2-2N-m^2}}\,. \tag{S46}$$

In the limit $N \to \infty$ where $N \gg m$, we see that the rational function in the square root approaches 1/3 and hence the critical bias becomes

$$\lim_{N\to\infty} |B_c| = \frac{1}{\sqrt{3}}\,. \tag{S47}$$

**Case 2: $N+m$ is odd**

In this case we require that

$$PLP(N-3) - PLP(N-1) > 0\,, \tag{S48}$$

where the first term is

$$PLP(N-3) = p^{\frac{N-m-3}{2}} q^{\frac{N+m-3}{2}}\binom{N-3}{\frac{N-m-3}{2}}S(3) = \frac{1}{2^N}\frac{(1-B^2)^{\frac{N}{2}}}{(1/4)^{\frac{3}{2}}(1-B^2)^{\frac{3}{2}}}\left(\frac{1-B}{1+B}\right)^{\frac{m}{2}}\binom{N-3}{\frac{N-m-3}{2}}S(3) \tag{S49}$$

and the second term is

$$PLP(N-1) = p^{\frac{N-m-1}{2}} q^{\frac{N+m-1}{2}}\binom{N-1}{\frac{N-m-1}{2}}S(1) = \frac{1}{2^N}\frac{(1-B^2)^{\frac{N}{2}}}{(1/4)^{\frac{1}{2}}(1-B^2)^{\frac{1}{2}}}\left(\frac{1-B}{1+B}\right)^{\frac{m}{2}}\binom{N-1}{\frac{N-m-1}{2}}S(1)\,. \tag{S50}$$

We can simplify these expressions using the fact that $S(1) = 1$ and $S(3) = S(2) = p^2 + q^2 = \frac{1}{2}(1+B^2)$. Finally, note that the two binomial coefficients $\binom{N-1}{\frac{N-m-1}{2}}$ and $\binom{N-3}{\frac{N-m-3}{2}}$ are related to each other as follows:

$$\binom{N-1}{\frac{N-m-1}{2}} = \frac{(N-1)(N-2)}{\left(\frac{N+m-1}{2}\right)\left(\frac{N-m-1}{2}\right)}\binom{N-3}{\frac{N-m-3}{2}}. \tag{S51}$$

Substituting these into Eq. S48 and canceling like terms yields the inequality

$$\frac{1+B^2}{1-B^2} > 2\frac{N^2-3N+2}{(N-1)^2-m^2} \tag{S52}$$

and solving for the bias $B$ gives the following:

$$B^2 > \frac{N^2 - 4N + 3 + m^2}{3N^2 - 8N + 5 - m^2} . \tag{S53}$$

We thus obtain the expression given in the main text:

$$|B| > \sqrt{\frac{N^2 - 4N + 3 + m^2}{3N^2 - 8N + 5 - m^2}} . \tag{S54}$$

The rational function inside the square root approaches 1/3 in the limit of infinite step number $N$. Thus, as before, we see that $B_c = 1/\sqrt{3}$ in the $N \to \infty$ limit when $N \gg m$.

# References


[1] S. Reuveni, "Catalan's Trapezoids," *Probability in the Engineering and Informational Sciences*, **28**(3), pp.353-361 (2014).

[2] D. Mookerjee and S. Kostinski. "Exact closed-form recurrence probabilities for biased random walks at any step number," *Europhysics Letters* **149**(6), p.62002 (2025).
